# Supplementary material for: Non Common Path Aberrations Correction
Source: arXiv:2211.00775 source file (2022-11-01)
Supplement: Supplementary file 1 [file fourier_optics_theory_appendix.tex]

\chapter{Electric Field Conjugation}

\relSection{coucou}

\relSection{Circulant Matrix}
